# Supplementary material for: IsoChronoMeter: A simple and effective isochronic translation evaluation metric
Source: arXiv:2410.11127 source file (2024-10-14)
Supplement: Supplementary file 1 [file appendix.tex]

\appendix
\section{System Papers}
\label{appendix}

\begin{itemize}
    \item ``{MSLC24} Submissions to the General Machine Translation Task'' \citep{wmt24_id2}
    \item ``{IOL} Research Machine Translation Systems for {WMT24} General Machine Translation Shared Task'' \citep{wmt24_id3}
    \item ``Choose the Final Translation from {NMT} and {LLM} Hypotheses Using {MBR} Decoding: {HW}-{TSC}'s Submission to the {WMT24} General {MT} Shared Task'' \citep{wmt24_id4}
    \item ``CycleGN: a Cycle Consistent approach for Neural Machine Translation'' \citep{wmt24_id5}
    \item ``UvA-{MT}'s Participation in the {WMT24} General Translation Shared Task'' \citep{wmt24_id6}
    \item ``Tower v2: Unbabel-{IST} 2023 Submission for the General {MT} Shared Task'' \citep{wmt24_id7}
    \item ``{CUNI}-{DS} submission: A Naive Transfer Learning Setup for English-to-Russian Translation Utilizing English-to-Czech Data'' \citep{wmt24_id10}
    \item ``{TSU} {HITS}'s Submissions to the {WMT} 2024 General Machine Translation Shared Task'' \citep{wmt24_id11}
    \item ``Hyper-{SNMT} at Translation Task'' \citep{wmt24_id13}
    \item ``Document-level Translation with {LLM} Reranking: Team-J at {WMT} 2024 General Translation Task'' \citep{wmt24_id14}
    \item ``{DLUT} and {GTCOM}'s Neural Machine Translation Systems for {WMT24}'' \citep{wmt24_id15}
    \item ``{CUNI} at {WMT24} General Translation Task: LLMs, (Q)LoRA, {CPO} and Model Merging'' \citep{wmt24_id17}
    \item ``From General {LLM} to Translation: How we dramatically improve translation quality using human evaluation data for {LLM} finetuning'' \citep{wmt24_id17}
    \item ``Cogs in a Machine, Doing What They're Meant to Do – The {AMI} Submission to the {WMT24} General Translation Task''\citep{wmt24_id18}
    \item ``{IKUN} for {WMT24} General {MT} Task: LLMs Are here for Multilingual Machine Translation'' \citep{wmt24_id19}
    \item ``{NTTSU} at {WMT2024} General Translation Task'' \citep{wmt24_id20}
    \item ``{SCIR}-{MT}'s Submission for {WMT24} General Machine Translation Task'' \citep{wmt24_id21}
    \item ``{AIST} {AIRC} Systems for the {WMT} 2024 Shared Tasks'' \citep{wmt24_id22}
    \item ``Occiglot at {WMT24}: European open-source large language models evaluated on translation'' \citep{wmt24_id23}
    \item ``English-to-Low-Resource Translation: A Multimodal Approach for Hindi, Malayalam, Bengali, and Hausa'' \citep{wmt24_id157}
\end{itemize}
